# Supplementary material for: NPC: Neural Point Characters from Video
Source: arXiv:2304.02013 source file (2023-09-01)
Supplement: Supplementary file 1 [file fig_canonical_points.tex]

\newlength\canonicalptsscale
\setlength\canonicalptsscale{0.27\textwidth}
\ifblurface
\newcommand{\canonicalptspost}{_blur}
\else
\newcommand{\canonicalptspost}{}
\fi
\newcommand{\canonicalptspath}{statics/figs/supp/initial_canonical/}
\newcommand{\canonicalptsma}{S1}%
\newcommand{\canonicalptsmb}{S5}%
\newcommand{\canonicalptsmc}{S6}%
\newcommand{\canonicalptsmd}{S7}%
\newcommand{\canonicalptsme}{S8}%
\newcommand{\canonicalptsmf}{S9}%
\newcommand{\canonicalptsmg}{S11}%
\newcommand{\canonicalptsmh}{weipeng}%
\newcommand{\canonicalptsmi}{nadia}%
\begin{figure*}[t]
\setlength{\fboxsep}{0pt}%
\setlength{\fboxrule}{0pt}%
\parbox[t]{\canonicalptsscale}{%
\centering%
\fbox{\includegraphics%
[width=\canonicalptsscale,trim=0 0 0 0,clip]%
{\canonicalptspath\canonicalptsma\canonicalptspost}%
}\\%
{Human3.6M \canonicalptsma}\\%
\fbox{\includegraphics%
[width=\canonicalptsscale,trim=0 0 0 0,clip]%
{\canonicalptspath\canonicalptsmd\canonicalptspost}%
}\\%
{Human3.6M \canonicalptsmd}\\%
\fbox{\includegraphics%
[width=\canonicalptsscale,trim=0 0 0 0,clip]%
{\canonicalptspath\canonicalptsmg\canonicalptspost}%
}\\%
{Human3.6M \canonicalptsmg}\\%
}%
\hfill%
\parbox[t]{\canonicalptsscale}{%
\centering%
\fbox{\includegraphics%
[width=\canonicalptsscale,trim=0 0 0 0,clip]%
{\canonicalptspath\canonicalptsmb\canonicalptspost}%
}\\%
{Human3.6M \canonicalptsmb}\\%
\fbox{\includegraphics%
[width=\canonicalptsscale,trim=0 0 0 0,clip]%
{\canonicalptspath\canonicalptsme\canonicalptspost}%
}\\%
{Human3.6M \canonicalptsme}\\%
\fbox{\includegraphics%
[width=\canonicalptsscale,trim=0 0 0 0,clip]%
{\canonicalptspath\canonicalptsmh\canonicalptspost}%
}\\%
{MonoPerfCap \canonicalptsmh}\\%
}%
\hfill%
\parbox[t]{\canonicalptsscale}{%
\centering%
\fbox{\includegraphics%
[width=\canonicalptsscale,trim=0 0 0 0,clip]%
{\canonicalptspath\canonicalptsmc\canonicalptspost}%
}\\%
{Human3.6M \canonicalptsmc}\\%
\fbox{\includegraphics%
[width=\canonicalptsscale,trim=0 0 0 0,clip]%
{\canonicalptspath\canonicalptsmf\canonicalptspost}%
}\\%
{Human3.6M \canonicalptsmf}\\%
\fbox{\includegraphics%
[width=\canonicalptsscale,trim=0 0 0 0,clip]%
{\canonicalptspath\canonicalptsmi\canonicalptspost}%
}\\%
{MonoPerfCap \canonicalptsmi}\\%
}%
\centering%
\caption{\textbf{Initial canonical point clouds extracted using DANBO~\cite{su2022danbo}.} Overall, DANBO can capture the rough geometry of the target character in about half an hour. These points serve as a good starting point for~\ourapproach{} to build details appearance on top.
}%
\label{fig:supp-initial-canonical}
\end{figure*}
