# Supplementary material for: NPC: Neural Point Characters from Video
Source: arXiv:2304.02013 source file (2023-09-01)
Supplement: Supplementary file 2 [file fig_limitation.tex]

\newlength\quallimitationscale
\setlength\quallimitationscale{0.33\linewidth}
\ifblurface
\newcommand{\quallimitationpost}{_blur}
\else
\newcommand{\quallimitationpost}{}
\fi
\newcommand{\quallimitationpath}{statics/figs/supp/limitation/}
\newcommand{\quallimitationma}{NeuralBody}
\newcommand{\quallimitationmb}{\phantom{(test)}ARAH\phantom{(test)}}
\newcommand{\quallimitationmc}{DANBO}
\newcommand{\quallimitationmd}{TAVA}
\newcommand{\quallimitationme}{NPC (Ours)}
\newcommand{\quallimitationa}{NeuralBody_00}
\newcommand{\quallimitationb}{ARAH_00}
\newcommand{\quallimitationc}{DANBO_00}
\newcommand{\quallimitationd}{TAVA_00}
\newcommand{\quallimitatione}{Ours-full_00}

\begin{figure}[h]
\setlength{\fboxsep}{0pt}%
\setlength{\fboxrule}{0pt}%
\parbox[t]{\quallimitationscale}{%
\centering%
\fbox{\includegraphics%
[width=\quallimitationscale,trim=0 0 0 80,clip]%
{\quallimitationpath GT_00\quallimitationpost}%
}\\%
{ Reference image}\\%
\fbox{\includegraphics%
[width=\quallimitationscale,trim=0 0 0 80,clip]%
{\quallimitationpath\quallimitationc\quallimitationpost}%
}\\%
{ \quallimitationmc}%
}%
\hfill%
\parbox[t]{\quallimitationscale}{%
\centering%
\fbox{\includegraphics%
[width=\quallimitationscale,trim=0 0 0 80,clip]%
{\quallimitationpath\quallimitationa\quallimitationpost}%
}\\%
{ \quallimitationma}\\%
\fbox{\includegraphics%
[width=\quallimitationscale,trim=0 0 0 80,clip]%
{\quallimitationpath\quallimitationd\quallimitationpost}%
}\\%
{ \quallimitationmd}%
}%
\hfill%
\parbox[t]{\quallimitationscale}{%
\centering%
\fbox{\includegraphics%
[width=\quallimitationscale,trim=0 0 0 80,clip]%
{\quallimitationpath\quallimitationb\quallimitationpost}%
}\\%
{ \quallimitationmb}\\%
\fbox{\includegraphics%
[width=\quallimitationscale,trim=0 0 0 80,clip]%
{\quallimitationpath\quallimitatione\quallimitationpost}%
}\\%
{ \quallimitationme}%
}%
\centering%
\caption{\textbf{Limitation.} While~\ourapproach{} retains sharp details on the cloth patterns, the sparse points cannot cover the stretched thigh sufficiently, resulting in ball-shaped artefacts.
}%
\label{fig:supp-limitation}
\end{figure}
