# Supplementary material for: NPC: Neural Point Characters from Video
Source: arXiv:2304.02013 source file (2023-09-01)
Supplement: Supplementary file 3 [file fig_monoperf.tex]

\newlength\monoperfscale
\setlength\monoperfscale{0.16\textwidth} %

\ifblurface
\newcommand{\monoperfpost}{_blur}
\else
\newcommand{\monoperfpost}{}
\fi
\setlength{\fboxsep}{0pt}%
\setlength{\fboxrule}{0pt}%
\parbox[t]{\monoperfscale}{%
\centering%
\fbox{\includegraphics%
[width=\monoperfscale,trim=0 0 250 0,clip]%
{statics/figs/supp/monoperf/nadia_GT_00\monoperfpost}%
}\\%
\fbox{\includegraphics%
[width=\monoperfscale,trim=0 0 220 0,clip]%
{statics/figs/supp/monoperf/weipeng_GT_00\monoperfpost}%
}\\%
{Ground truth}%
}%
\hfill%
\parbox[t]{\monoperfscale}{%
\centering%
\fbox{\includegraphics%
[width=\monoperfscale,trim=0 0 250 0,clip]
{statics/figs/supp/monoperf/nadia_DANBO_00\monoperfpost}%
}\\%
\fbox{\includegraphics%
[width=\monoperfscale,trim=0 0 220 0,clip]%
{statics/figs/supp/monoperf/weipeng_DANBO_00\monoperfpost}%
}\\%
{DANBO}%
}%
\hfill
\parbox[t]{\monoperfscale}{%
\centering%
\fbox{\includegraphics%
[width=\monoperfscale,trim=0 0 250 0,clip]%
{statics/figs/supp/monoperf/nadia_NPC_00\monoperfpost}%
}\\%
\fbox{\includegraphics%
[width=\monoperfscale,trim=0 0 220 0,clip]%
{statics/figs/supp/monoperf/weipeng_NPC_00\monoperfpost}%
}\\%
{NPC (Ours)}%
}%
\hfill
\parbox[t]{\monoperfscale}{%
\centering%
\fbox{\includegraphics%
[width=\monoperfscale,trim=0 0 250 0,clip]%
{statics/figs/supp/monoperf/nadia_GT_01\monoperfpost}%
}\\%
\fbox{\includegraphics%
[width=\monoperfscale,trim=30 0 147 0,clip]%
{statics/figs/supp/monoperf/weipeng_GT_01}%
}\\%
{Ground truth}%
}%
\hfill%
\parbox[t]{\monoperfscale}{%
\centering%
\fbox{\includegraphics%
[width=\monoperfscale,trim=0 0 250 0,clip]%
{statics/figs/supp/monoperf/nadia_DANBO_01\monoperfpost}%
}\\%
\fbox{\includegraphics%
[width=\monoperfscale,trim=30 0 147 0,clip]%
{statics/figs/supp/monoperf/weipeng_DANBO_01}%
}\\%
{DANBO}%
}%
\hfill
\parbox[t]{\monoperfscale}{%
\centering%
\fbox{\includegraphics%
[width=\monoperfscale,trim=0 0 250 0,clip]%
{statics/figs/supp/monoperf/nadia_NPC_01\monoperfpost}%
}\\%
\fbox{\includegraphics%
[width=\monoperfscale,trim=30 0 147 0,clip]%
{statics/figs/supp/monoperf/weipeng_NPC_01}%
}\\%
{NPC (Ours)}%
}%
\centering%
\captionof{figure}{\textbf{Unseen pose rendering from MonoPerfCap~\cite{Xu18a} test split}. Similar to the unseen pose synthesis results on Human3.6M~\cite{Ionescu11,Ionescu14a},~\ourapproach{} produces sharper and more plausible details, such as shoes, knuckles, and ears. \vspace{0.3cm}}%
\label{fig:supp-monoperf-novel-pose}
