# Supplementary material for: NPC: Neural Point Characters from Video
Source: arXiv:2304.02013 source file (2023-09-01)
Supplement: Supplementary file 4 [file fig_architecture.tex]

\newlength\supparchiscale
\setlength\supparchiscale{0.33\textwidth}
\begin{figure*}[h]
\setlength{\fboxsep}{0pt}%
\setlength{\fboxrule}{0pt}%
\centering%
\parbox[t]{\supparchiscale}{%
\centering%
\fbox{%
\includegraphics[width=0.5\supparchiscale,trim=00 0 55 0,clip]{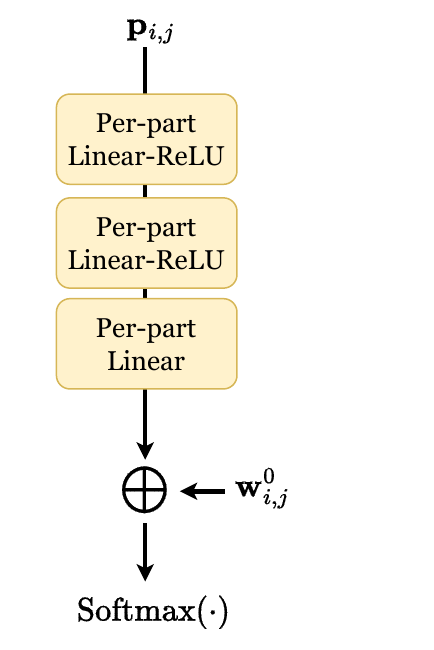}%
}\\%
{(a) Linear blend skinning network $\text{MLP}_{\vw,j}$ }%
}%
\hfill%
\parbox[t]{\supparchiscale}{%
\centering%
\fbox{%
\includegraphics[width=0.58\supparchiscale,trim=20 0 25 0,clip]{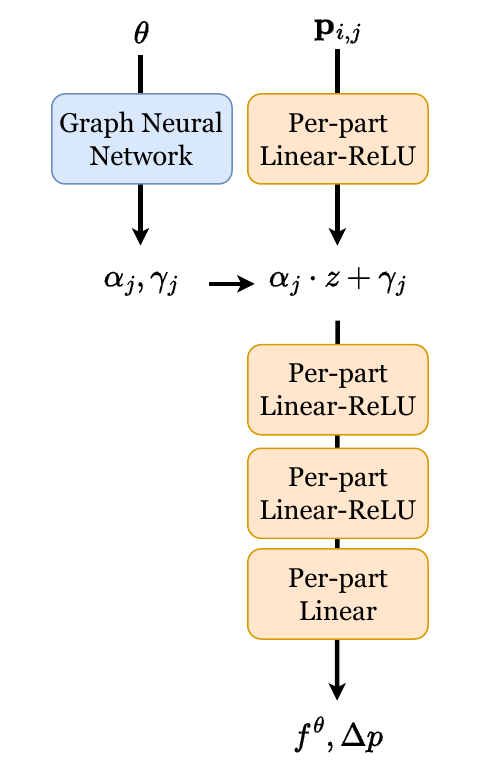}%
}\\%
{(b) GNN-FiLM }%
}%
\hfill%
\parbox[t]{\supparchiscale}{%
\centering%
\fbox{%
\includegraphics[width=0.9\supparchiscale,trim=60 0 0 0,clip]{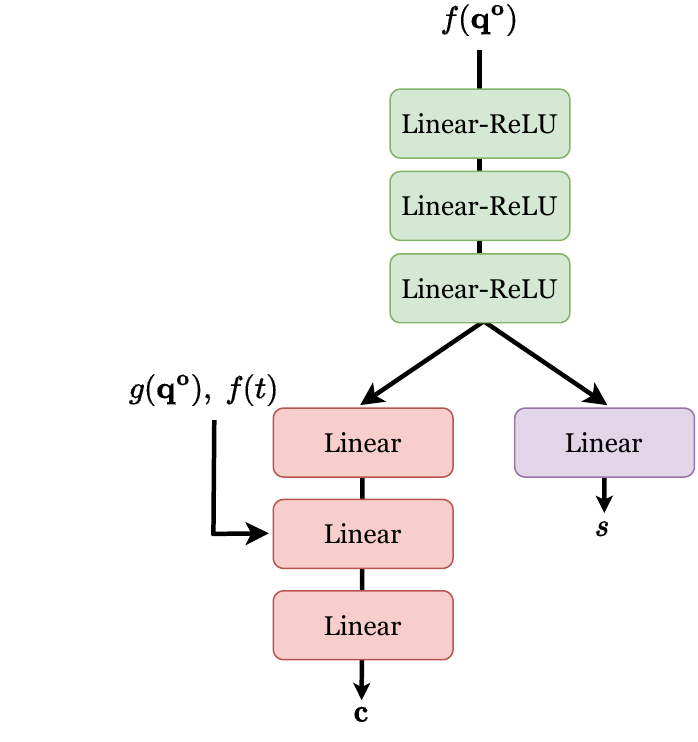}%
}\\%
{(c) NeRF $F_\psi$ }%
}%
\centering%
\caption{\textbf{Network architectures.} (a) We use a small MLP for each body part to predict the residual of the initial LBS weights $\vw^0_{i,j}$, producing the final weight. (b) Our GNN predicts conditional vectors local to each body part for modulating the pose dependent outputs. (c) Our NeRF $F_\psi$ is modified from the original architecture~\cite{mildenhall2020nerf}, with less shared layer (green). Our character-specific features $f(\vq^\vo), g(\vq^\vo),$ and $f(t)$ are introduced at two different layers to maintain view direction invariance for predicting $s$.}%
\label{fig:supp-architecture}
\end{figure*}
