# Supplementary material for: NPC: Neural Point Characters from Video
Source: arXiv:2304.02013 source file (2023-09-01)
Supplement: Supplementary file 5 [file fig_full_h36m_novel_pose.tex]

\newlength\hmqualscale
\setlength\hmqualscale{0.160\textwidth} %
\newcommand{\hmqualpath}{statics/figs/exp/h36m_novelpose/}
\ifblurface
\newcommand{\hmqualpost}{_blur}
\else
\newcommand{\hmqualpost}{}
\fi
\newcommand{\hmqualma}{NeuralBody}
\newcommand{\hmqualmb}{ARAH}
\newcommand{\hmqualmc}{DANBO}
\newcommand{\hmqualmd}{TAVA}
\newcommand{\hmqualme}{Ours-full}
\newcommand{\hmquala}{S6}
\newcommand{\hmqualanum}{00}
\newcommand{\hmquale}{S7}
\newcommand{\hmqualenum}{00}
\newcommand{\hmqualf}{S8}
\newcommand{\hmqualfnum}{00}
\newcommand{\hmqualg}{S6}
\newcommand{\hmqualgnum}{01}
\newcommand{\hmqualh}{S7}
\newcommand{\hmqualhnum}{01}
\begin{figure*}[!h]
\setlength{\fboxsep}{0pt}%
\setlength{\fboxrule}{0pt}%
\parbox[t]{\hmqualscale}{%
\centering%
\fbox{\includegraphics%
[width=\hmqualscale]
{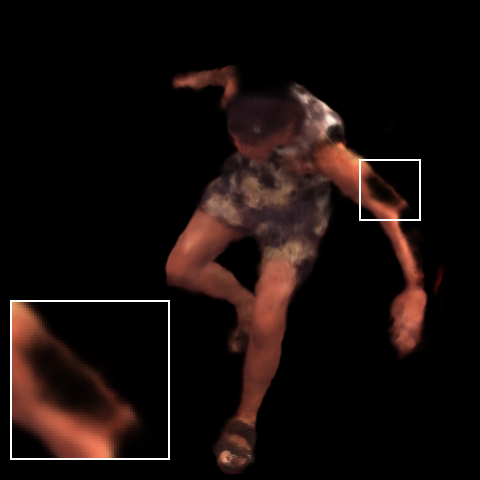}%
}\\%
\fbox{\includegraphics%
[width=\hmqualscale]
{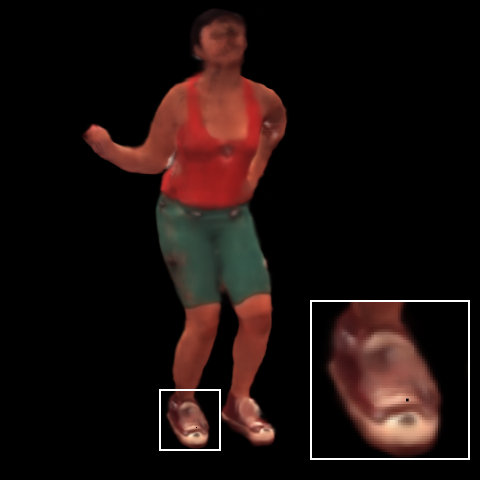}%
}\\%
\fbox{\includegraphics%
[width=\hmqualscale]
{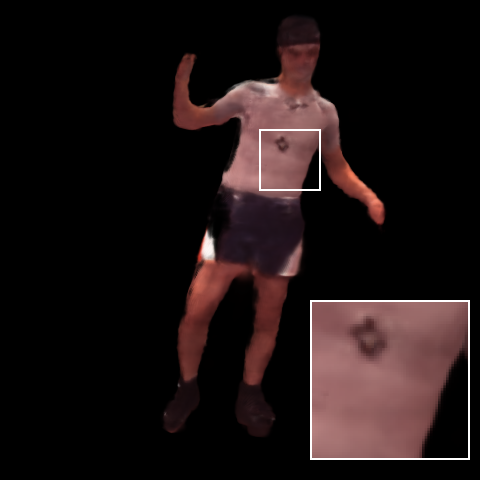}%
}\\%
\fbox{\includegraphics%
[width=\hmqualscale]
{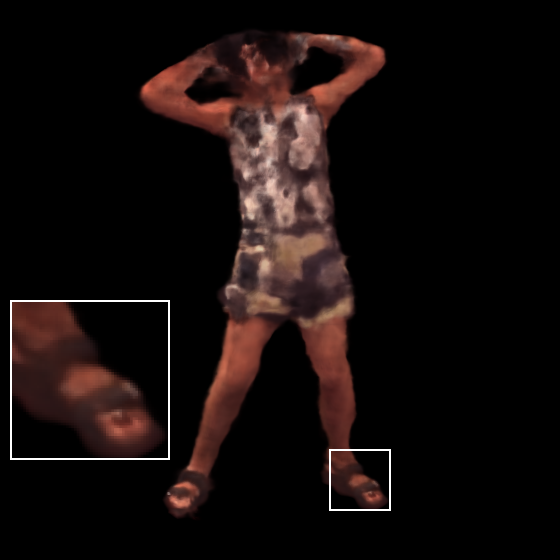}%
}\\%
\fbox{\includegraphics%
[width=\hmqualscale]
{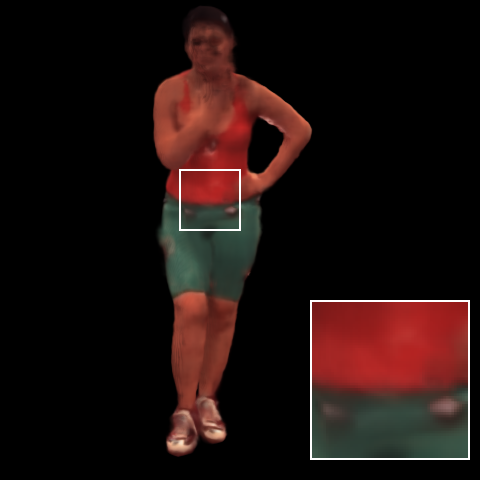}%
}\\%
{ \hmqualma}%
}%
\hfill%
\parbox[t]{\hmqualscale}{%
\centering%
\fbox{\includegraphics%
[width=\hmqualscale]
{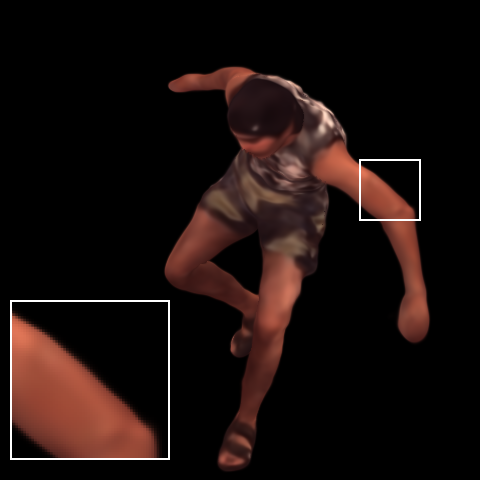}%
}\\%
\fbox{\includegraphics%
[width=\hmqualscale]
{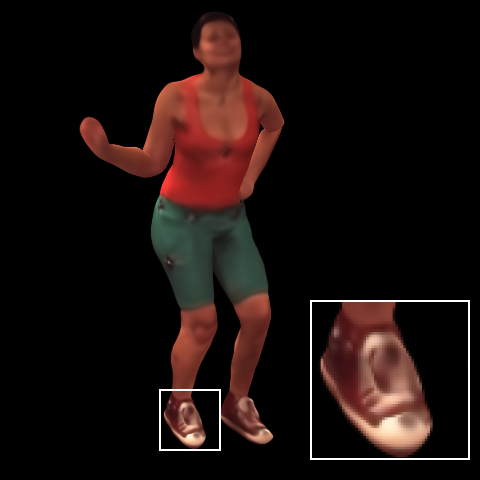}%
}\\%
\fbox{\includegraphics%
[width=\hmqualscale]
{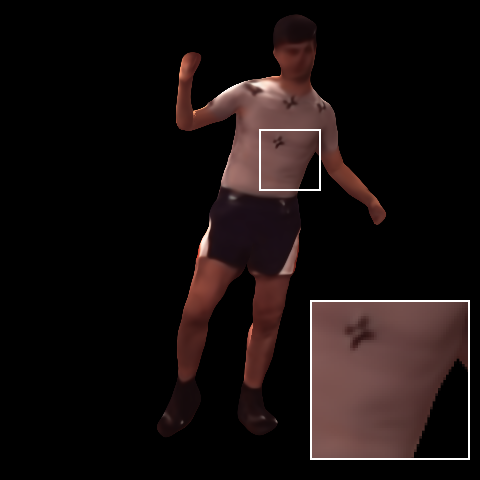}%
}\\%
\fbox{\includegraphics%
[width=\hmqualscale]
{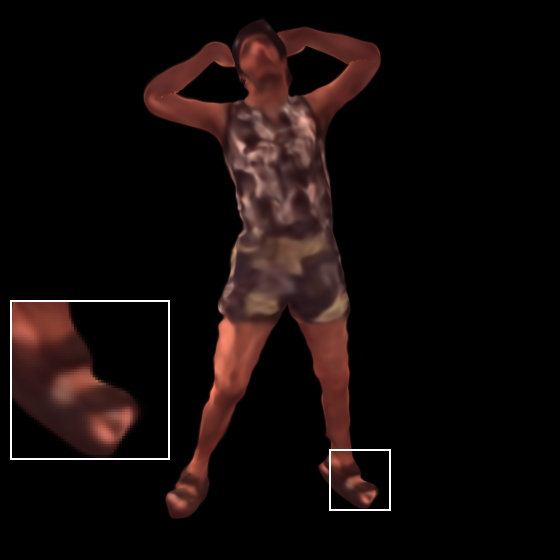}%
}\\%
\fbox{\includegraphics%
[width=\hmqualscale]
{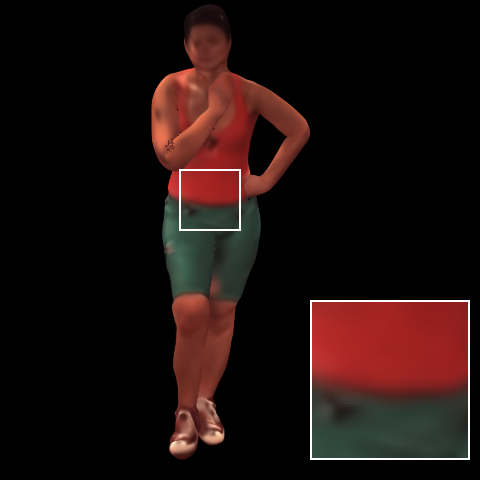}%
}\\%
{ \hmqualmb}%
}%
\hfill
\parbox[t]{\hmqualscale}{%
\centering%
\fbox{\includegraphics%
[width=\hmqualscale]
{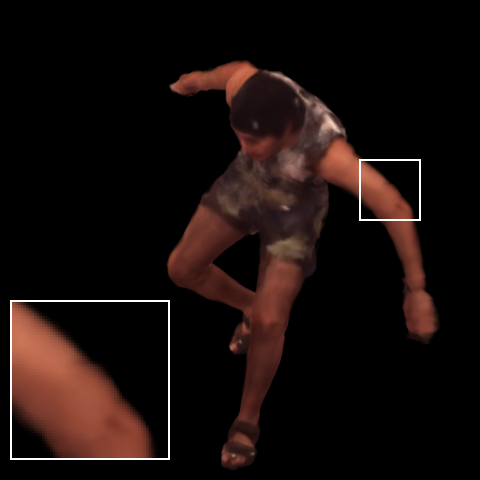}%
}\\%
\fbox{\includegraphics%
[width=\hmqualscale]
{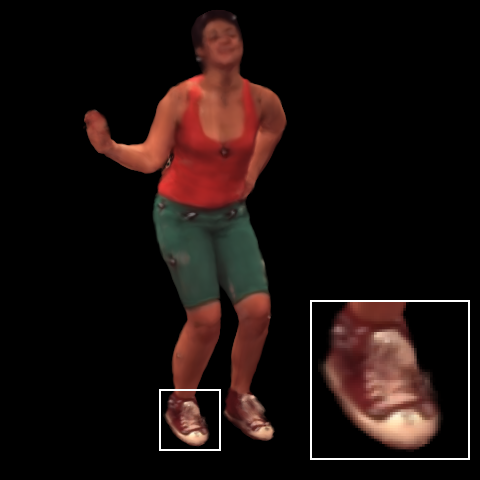}%
}\\%
\fbox{\includegraphics%
[width=\hmqualscale]
{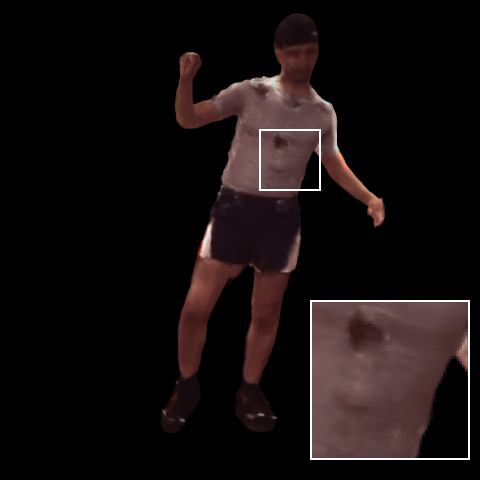}%
}\\%
\fbox{\includegraphics%
[width=\hmqualscale]
{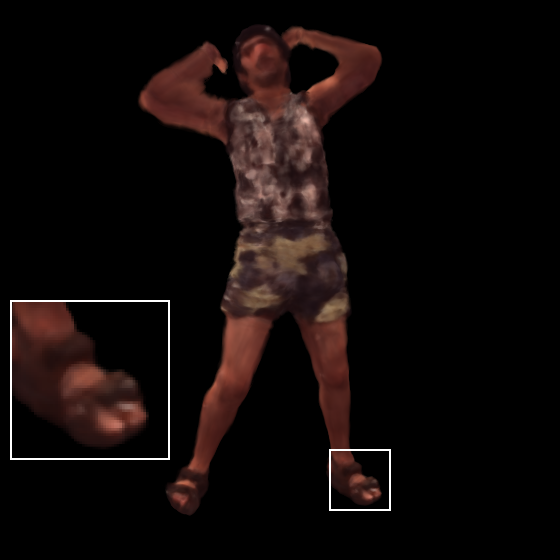}%
}\\%
\fbox{\includegraphics%
[width=\hmqualscale]
{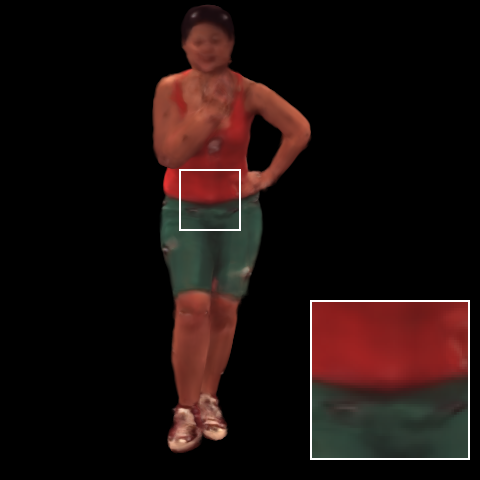}%
}\\%
{ \hmqualmc}%
}%
\hfill
\parbox[t]{\hmqualscale}{%
\centering%
\fbox{\includegraphics%
[width=\hmqualscale]
{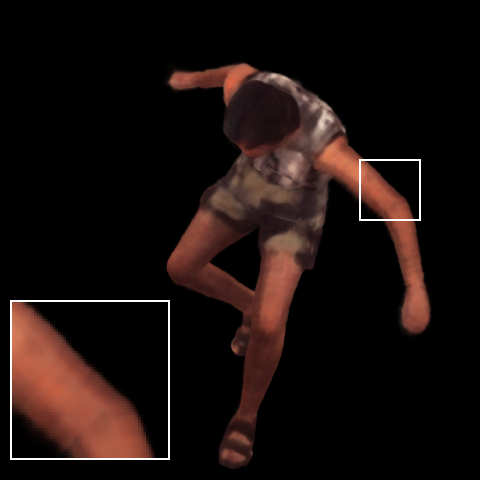}%
}\\%
\fbox{\includegraphics%
[width=\hmqualscale]
{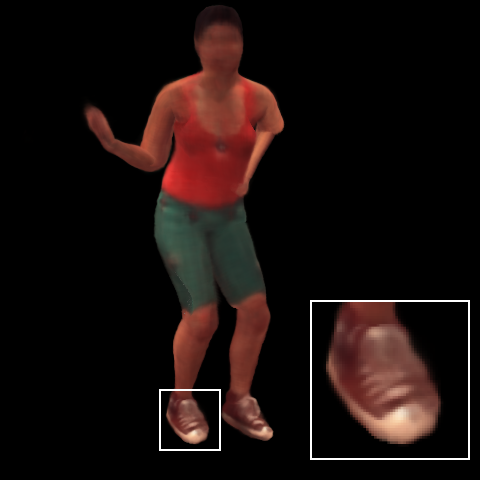}%
}\\%
\fbox{\includegraphics%
[width=\hmqualscale]
{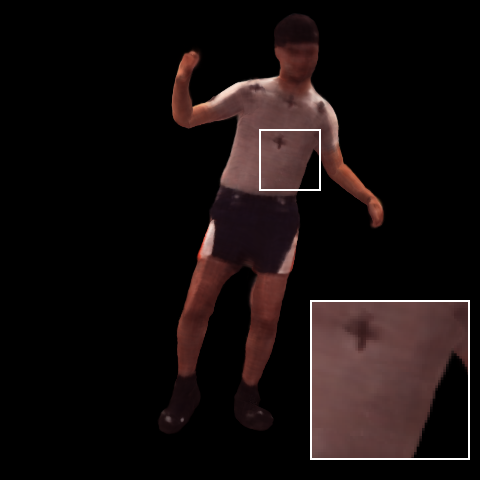}%
}\\%
\fbox{\includegraphics%
[width=\hmqualscale]
{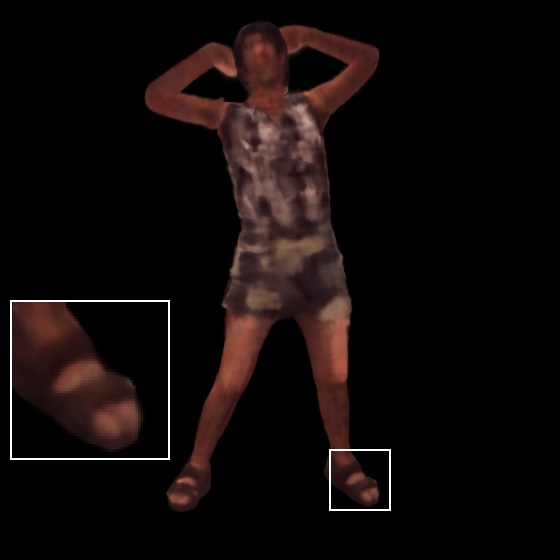}%
}\\%
\fbox{\includegraphics%
[width=\hmqualscale]
{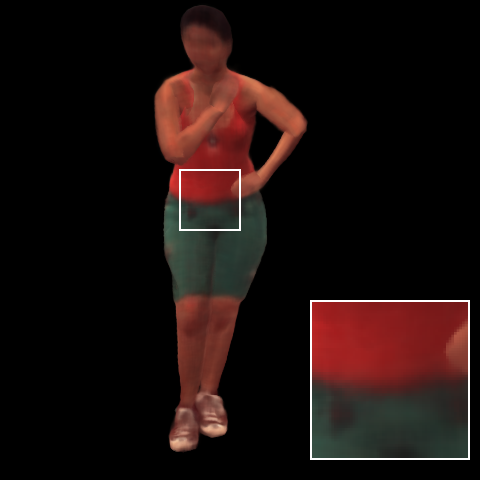}%
}\\%
{ \hmqualmd}%
}%
\hfill%
\parbox[t]{\hmqualscale}{%
\centering%
\fbox{\includegraphics%
[width=\hmqualscale]
{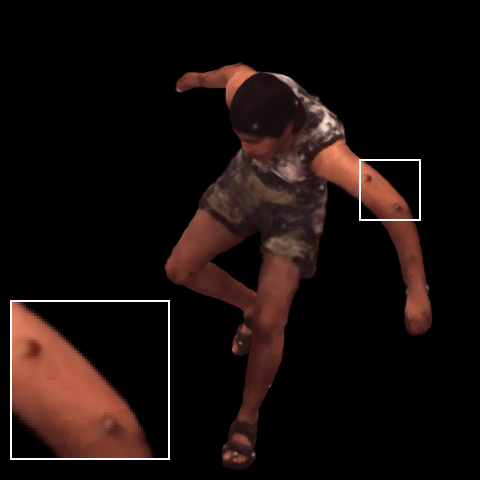}%
}\\%
\fbox{\includegraphics%
[width=\hmqualscale]
{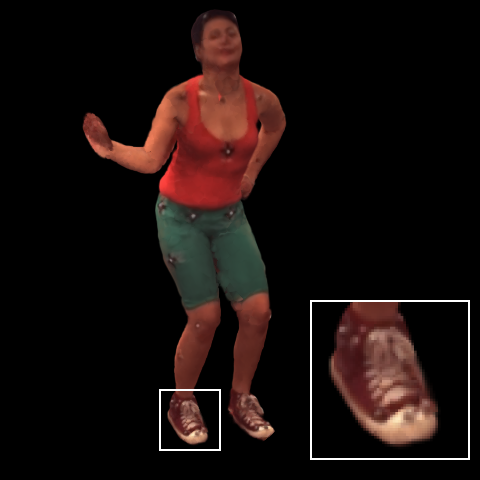}%
}\\%
\fbox{\includegraphics%
[width=\hmqualscale]
{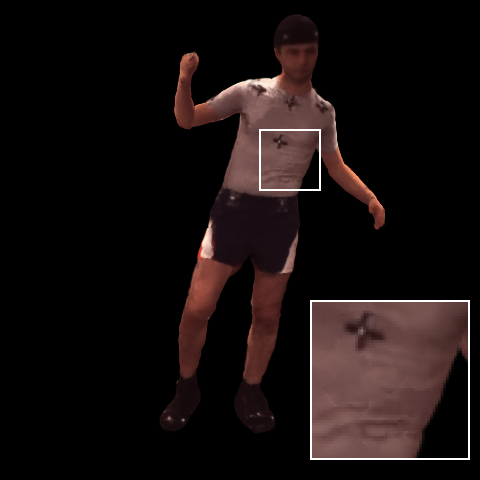}%
}\\%
\fbox{\includegraphics%
[width=\hmqualscale]
{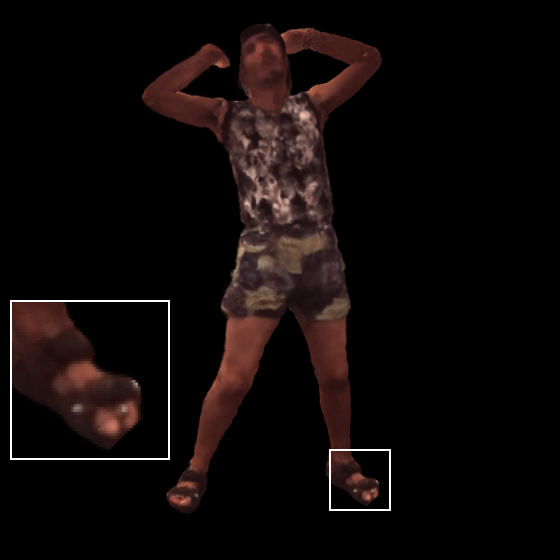}%
}\\%
\fbox{\includegraphics%
[width=\hmqualscale]
{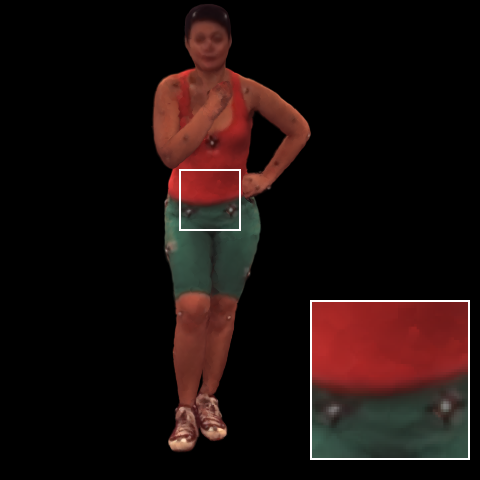}%
}\\%
{\ourapproach~(Ours)}
}%
\hfill
\parbox[t]{\hmqualscale}{%
\centering%
\fbox{\includegraphics%
[width=\hmqualscale]
{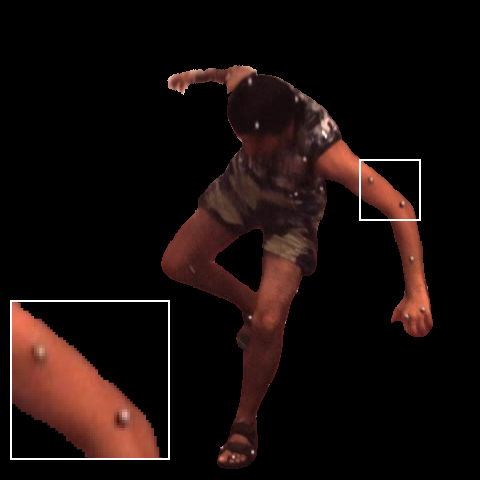}%
}\\%
\fbox{\includegraphics%
[width=\hmqualscale]
{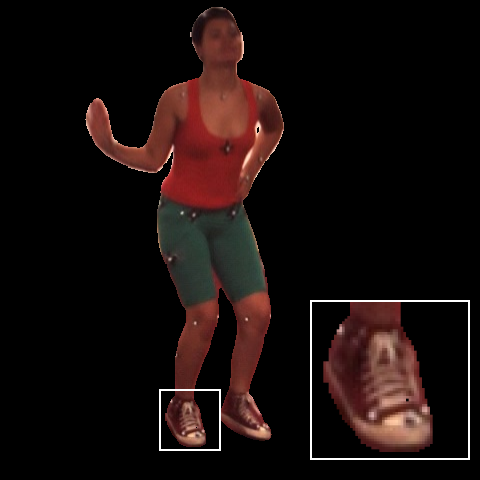}%
}\\%
\fbox{\includegraphics%
[width=\hmqualscale]
{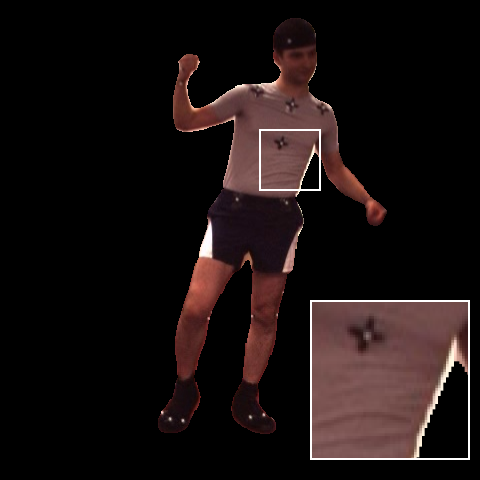}%
}\\%
\fbox{\includegraphics%
[width=\hmqualscale]
{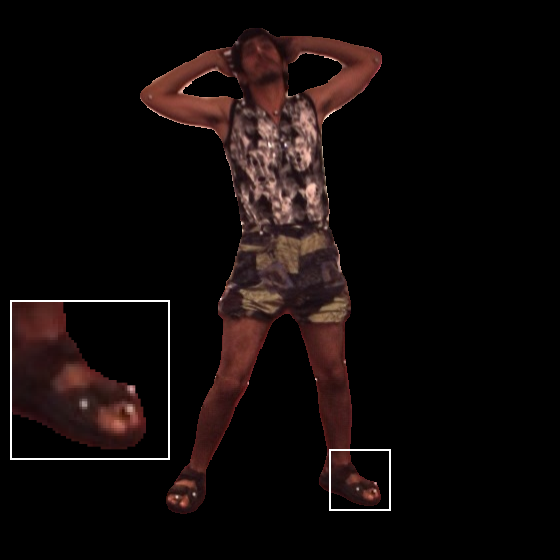}%
}\\%
\fbox{\includegraphics%
[width=\hmqualscale]
{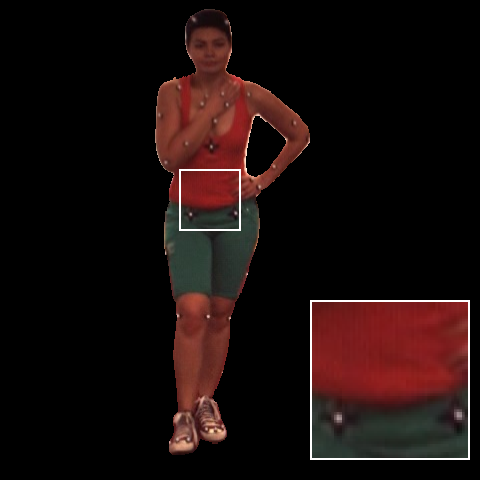}%
}\\%
{ Ground truth}%
}%
\centering%
\caption{\textbf{Unseen pose synthesis on Anim-NeRF Human3.6M~\cite{Ionescu11,Ionescu14a,peng2021animatable} test split}. On various subjects, \ourapproach{} shows better details in shoes, cloth wrinkles and body landmarks like motion capture trackers.
}%
\label{fig:supp-full-qualitative-novel-pose}
\end{figure*}
