# Supplementary material for: NPC: Neural Point Characters from Video
Source: arXiv:2304.02013 source file (2023-09-01)
Supplement: Supplementary file 7 [file table_supp_NN_search.tex]

\begin{table}[t]
\caption{\textbf{Tabulated K-NN overlaps with the naive K-NN with high probability}. We report the neighbor overlap rate between ours and the naive K-NN for $k=8$  , as well as the coverage rate of the $k$-th naive nearest neighbors.}
\centering
\resizebox{1.0\linewidth}{!}{
\setlength{\tabcolsep}{3pt}
\begin{tabular}{cccccc}
\toprule
1st & 2nd & 3rd & 4th & 5th & Overlap rate (all eight)\\
\midrule%
\rowcolor{Gray}
100\% & 86.4\% & 81.5\% & 75.9\% & 69.9\% & 72.6\% 
\end{tabular}
\label{tab:supp-nn-search}
}
\end{table}
