# Supplementary material for: NPC: Neural Point Characters from Video
Source: arXiv:2304.02013 source file (2023-09-01)
Supplement: Supplementary file 8 [file table_supp_SMPL_init.tex]

\begin{table}[t]
\caption{\ourapproach{} can also use SMPL~\cite{loper2015smpl} surface points for initialization.}
\centering
\resizebox{0.8\linewidth}{!}{
\setlength{\tabcolsep}{3pt}
\begin{tabular}{lcc}
\toprule
 & PSNR~$\uparrow$  & LPIPS~$\downarrow$  \\
\midrule
 \rowcolor{Gray}
DANBO init. & 24.86 (+0.00\%) & 0.115 (+0.00\%) \\
SMPL init. & 24.90 ({\color{green}+0.02\%})&  0.116 ({\color{red}+0.90\%}) \\
\end{tabular}
\label{tab:supp-smpl-init}
}
\end{table}
