# Supplementary material for: NPC: Neural Point Characters from Video
Source: arXiv:2304.02013 source file (2023-09-01)
Supplement: Supplementary file 9 [file table_supp_full_ablation.tex]

\begin{table}[t]
\caption{\textbf{Ablation study on each of our proposed designs.} Most of our features contribute to the final perceptual quality.}
\centering
\resizebox{0.75\linewidth}{!}{
\setlength{\tabcolsep}{3pt}
\begin{tabular}{lccccc}
\toprule
 & KIDx100~$\downarrow$  & LPIPS (VGG)~$\downarrow$ & LPIPS (Alex)~$\downarrow$ \\
\midrule
No $f^d$ & 5.54& 0.122 & 0.132\\
\rowcolor{Gray}
No $f^p$& 4.51& 0.122 & 0.131\\
No $f^\theta$& 4.50& 0.120 & 0.132\\
\rowcolor{Gray}
No $\Delta p$& 4.61& 0.120 & 0.131\\
No $f^v$ & 4.48&  0.115 & \textbf{0.124}\\
\rowcolor{Gray}
No $r_i$& \textbf{3.87}& 0.116 &  0.125\\
\midrule%
\textbf{Ours full}& 4.43 & \textbf{0.115} & \textbf{0.124}\\
\end{tabular}
\label{tab:supp-ablation}
}
\end{table}
